# Supplementary material for: Boltzmann Exploration Expectation-Maximisation
Source: arXiv:1912.08869 source file (2019-12-18)
Supplement: Supplementary file 1 [file gmm_experiments_appendix.tex]

\section{Gaussian mixture model addendum}
\label{sec:gmm_appendix}
\FloatBarrier

The plots in \cref{fig:gmm_mixture_figs} relate to the experiments conducted in \cref{sec:GMM_experiments}.

\input{figures/gmm_mixture_fig.tex}
